# Supplementary material for: A Thorough Examination of Decoding Methods in the Era of LLMs
Source: arXiv:2402.06925 source file (2024-10-08)
Supplement: Supplementary file 1 [file appendix-factscore-prompt.tex]

\begin{table*}[h]
    \centering
    \small
    \begin{tabular}{p{\linewidth}}
        \toprule
        \underline{\textbf{\textsc{Prompt for FActSore}}} \\
        \vspace{-2mm}
        \textbf{Question:} Tell me a bio of \texttt{\textcolor{PERSON}{[ARTICLE]}}\\
        \bottomrule
    \end{tabular}
    \caption{0-shot prompt for FActSore (aligned model).}
    \label{tab:appendix-factscore-nochat-prompt}
\end{table*}
